# Supplementary material for: Quantum many-body scars as remnants of stable many-body periodic orbits
Source: arXiv:2410.16916 source file (2024-10-23)
Supplement: Supplementary file 1 [file appendix_new.tex]

%\clearpage
%\clearpage
\onecolumngrid
%\begin{center}
%\textbf{\large Supplemental material for ``Origin of long-lived oscillations in a Rydberg-blockaded chain: Projected precession of a large pseudospin"}\\
%\vspace{5mm}
%Keita Omiya$^{1,2,3}$ and Markus M\"uller$^2$\\
%\vspace{2.5mm}
%$^1$\textit{Department of Physics, ETH Z\"urich, CH-8093 Z\"urich, Switzerland}\\
%$^2$\textit{Condensed Matter Theory Group, LSM, NES, Paul Scherrer Institute, Villigen PSI, CH-5352, Switzerland}\\
%$^3$\textit{Institute of Physics, Ecole Polytechnique F\'ed\'erale de Lausanne (EPFL), CH-1015 Lausanne, Switzerland}
%\end{center}
%%%%%%%%%% Merge with supplemental materials %%%%%%%%%%
%%%%%%%%%% Prefix a "S" to all equations, figures, tables and reset the counter %%%%%%%%%%
%\setcounter{equation}{0}
%\setcounter{figure}{0}
%\setcounter{table}{0}
%\setcounter{page}{1}
%\makeatletter
%\renewcommand{\theequation}{S\arabic{equation}}
%\renewcommand{\thefigure}{S\arabic{figure}}
%\renewcommand{\bibnumfmt}[1]{[S#1]}
%\renewcommand{\citenumfont}[1]{S#1}
\section{Proof of the dimerization invariance of $\ket*{S_n}$ on bipartite lattices}\label{sec:invariance}
Here we show the dimerization invariance of our trial wavefunctions $\ket*{S_n}$,
%with respect to translations by one original $S=1/2$ site.
\begin{equation}\label{eq:SM |Sn>}
    \ket*{S_n}=P_{\mr{Ryd}}\left(\what{J}^-\right)^{N-n}\bigotimes_{b\in\Lambda_{\mr{B}}}\ket*{\what{+}}_b,
\end{equation}
where $\what{J}^\pm=\mp i\sum_{b\in\Lambda_{\mr{B}}}(S_b^y\pm iS_b^z)$ is the collective ladder operator defined in the main text.  

To show the above, we will transform the action of $J^-$ on the block spin into a form that acts individually on the $S=1/2$ degrees of freedom, cf. Eq.~(\ref{eq:from x basis to varphi compact}) below. From this we will infer that for all $k$ the action of $(J^-)^k$  can be written as a product of dimerization invariant operators within the constrained subspace, which proves the dimerization invariance of $\ket*{S_n}$.

One can express the basis $\ket*{\what{\pm}}$ and $\ket*{\what{0}}$ in terms of wavefunctions of the two constituting $S=1/2$ spins as follows: 
\begin{equation}\label{eq:from x basis to S=1/2}
    \begin{split}
        \ket*{\what{+}}_b&=\frac{1}{2}\ket*{+}_b+\frac{1}{\sqrt{2}}\ket*{0}_b+\frac{1}{2}\ket*{-}_b=\frac{1}{2}\ket*{\downarrow\uparrow}_{b_\alpha,b_\beta}+\frac{1}{\sqrt{2}}\ket*{\downarrow\downarrow}_{b_\alpha,b_\beta}+\frac{1}{2}\ket*{\uparrow\downarrow}_{b_\alpha,b_\beta}\\
        \ket*{\what{0}}_b&=\frac{1}{\sqrt{2}}\ket*{+}_b-\frac{1}{\sqrt{2}}\ket*{-}_b=\frac{1}{\sqrt{2}}\ket*{\downarrow\uparrow}_{b_\alpha,b_\beta}-\frac{1}{\sqrt{2}}\ket*{\uparrow\downarrow}_{b_\alpha,b_\beta}\\
        \ket*{\what{-}}_b&=\frac{1}{2}\ket*{+}_b-\frac{1}{\sqrt{2}}\ket*{0}_b+\frac{1}{2}\ket*{-}_b=\frac{1}{2}\ket*{\downarrow\uparrow}_{b_\alpha,b_\beta}-\frac{1}{\sqrt{2}}\ket*{\downarrow\downarrow}_{b_\alpha,b_\beta}+\frac{1}{2}\ket*{\uparrow\downarrow}_{b_\alpha,b_\beta}.
    \end{split}
\end{equation}
The lowering operator $J_b^-\coloneqq\sqrt{2}(\dyad*{\what{0}}{\what{+}}+\dyad*{\what{-}}{\what{0}})_b$, which satisfies $\sum_{b\in\Lambda_{\mr{B}}}J_b^-=J^-$, 
can be used to write $\ket*{\what{0}}_b=\frac{1}{\sqrt{2}}J^-_b\ket*{\what{+}}_b$ and $\ket*{\what{-}}_b=\left(\frac{1}{\sqrt{2}}J^-_b\right)^2\ket*{\what{+}}_b$.

To re-write Eq.~\eqref{eq:from x basis to S=1/2}, and thus the action of $J_b^-$, in a translationally invariant manner, we introduce a new non-orthogonal basis of $S=1/2$ states, and an associated basis transformation $U^\varphi$:
\begin{equation}\begin{split}
    \ket*{\varphi}_i&\coloneqq\cos\varphi\ket*{\uparrow}_i+\sin\varphi\ket*{\downarrow}_i,\,\,\ket*{-\varphi}_i\coloneqq\cos\varphi\ket*{\uparrow}_i-\sin\varphi\ket*{\downarrow}_i,\,\,\varphi\coloneqq\arctan\sqrt{2},\\
    U_i^\varphi&\coloneqq\dyad*{\varphi}{\uparrow}_i+\dyad*{-\varphi}{\downarrow}_i.
    \end{split}
\end{equation}
With this basis, Eq.~\eqref{eq:from x basis to S=1/2} can be written as follows:
\begin{equation}\label{eq:from x basis to varphi}\begin{split}
    \ket*{\what{+}}_b&=\frac{3}{2\sqrt{2}}(1-\dyad*{\uparrow\uparrow})_{b_\alpha, b_\beta}\ket*{\varphi}_{b_\alpha}\ket*{\varphi}_{b_\beta}\\&=\frac{3}{2\sqrt{2}}(1-\dyad*{\uparrow\uparrow})_{b_\alpha, b_\beta}U^\varphi_{b_\alpha}U^\varphi_{b_\beta}\ket*{\uparrow\uparrow}_{b_\alpha, b_\beta}\\
    \ket*{\what{0}}_b&=\frac{3}{2\sqrt{2}}(1-\dyad*{\uparrow\uparrow})_{b_\alpha, b_\beta}\frac{1}{\sqrt{2}}\left(\ket*{\varphi}_{b_\alpha}\ket*{-\varphi}_{b_\beta}-\ket*{-\varphi}_{b_\alpha}\ket*{\varphi}_{b_\beta}\right)\\
    &=\frac{3}{2\sqrt{2}}(1-\dyad*{\uparrow\uparrow})_{b_\alpha, b_\beta}U_{b_\alpha}^\varphi U^\varphi_{b_\beta}\frac{1}{\sqrt{2}}\left(\ket*{\uparrow\downarrow}-\ket*{\downarrow\uparrow}\right)_{b_\alpha, b_\beta}\\
    &=\frac{3}{2\sqrt{2}}(1-\dyad*{\uparrow\uparrow})_{b_\alpha, b_\beta}U_{b_\alpha}^\varphi U^\varphi_{b_\beta}\frac{1}{\sqrt{2}}\left(-\sigma_{b_\alpha}^-+\sigma_{b_\beta}^-\right)\ket*{\uparrow\uparrow}_{b_\alpha, b_\beta}\\
    \ket*{\what{-}}_b&=\frac{3}{2\sqrt{2}}(1-\dyad*{\uparrow\uparrow})_{b_\alpha, b_\beta}\left(-\ket*{-\varphi}_{b_\alpha}\ket*{-\varphi}_{b_\beta}\right)\\&=\frac{3}{2\sqrt{2}}(1-\dyad*{\uparrow\uparrow})_{b_\alpha, b_\beta}U^\varphi_{b_\alpha}U^\varphi_{b_\beta}(-\ket*{\downarrow\downarrow}_{b_\alpha, b_\beta})\\
    &=\frac{3}{2\sqrt{2}}(1-\dyad*{\uparrow\uparrow})_{b_\alpha, b_\beta}U_{b_\alpha}^\varphi U^\varphi_{b_\beta}\left(\frac{1}{\sqrt{2}}(-\sigma_{b_\alpha}^-+\sigma_{b_\beta}^-)\right)^2\ket*{\uparrow\uparrow}_{b_\alpha, b_\beta}.
    \end{split}
\end{equation}
These results can be summarized in the following compact form: 
\begin{equation}
\label{eq:from x basis to varphi compact}
(J^-)^k \ket*{\what{+}}_b = \frac{3}{2\sqrt{2}}(1-\dyad*{\uparrow\uparrow})_{b_\alpha, b_\beta}U_{b_\alpha}^\varphi U^\varphi_{b_\beta}\left(-\sigma_{b_\alpha}^-+\sigma_{b_\beta}^-\right)^k\ket*{\uparrow\uparrow}_{b_\alpha, b_\beta},
\end{equation}
which holds for all $k\geq 0$

Using Eq.~\eqref{eq:from x basis to varphi compact} in %\MM{no, not in (D2), but in the (so far absent) definition of $S_n$.}
Eq.~\eqref{eq:SM |Sn>}, one immediately obtains
\begin{equation}\label{eq:manifest inv Sn}
    \ket*{S_n}=\left(\frac{3}{2\sqrt{2}}\right)^NP_{\mr{Ryd}}\prod_{i\in\Lambda}U_i^\varphi\left(\sum_{j\in\Lambda_\alpha}\sigma_j^-{-\sum_{j'\in\Lambda_\beta}\sigma^-_{j'}}\right)^{N-n}\bigotimes_{k\in\Lambda}\ket*{\uparrow}_k,
\end{equation}
which  is manifestly independent of the choice of dimers. 
%the transformation under translation, Eq.~\eqref{eq:main claim}, can easily be read off.

For the Rydberg chain, let $T$ be the translation operator.  The above explicit form of $\ket*{S_n}$ shows that
\begin{equation}\label{eq:main claim}
    T\ket*{S_n}=(-1)^{N-n}\ket*{S_n},
\end{equation}
expressing the fact that the trial scar states carry total lattice momentum $(N-n)\pi$ (modulo $2\pi$). 

\section{{Restoring lattice symmetries of non-Hermitian perturbations}}
\label{sec:appendix inv perturbation}
{In this section, we show that the non-Hermitian perturbations constructed in Sec.~\ref{sec:perturbation} can be modified so as to restore symmetries of the original Hamiltonian. We start from the following almost trivial observation: if $\ket*{S_n}$ is an eigenstate of $H+\delta H_{\mr{NH}}$ with eigenvalue $E_n$, 
%if the Hamiltonian commutes with a certain symmetry operation $g$, i.e., $[H,g]=0$ for $\forall g\in G$, 
and if $\ket*{S_n}$ is invariant under $g$, i.e., $O_g\ket*{S_n}=\alpha_g\ket*{S_n}$ with a simple phase factor $\alpha_g$, then $\ket*{S_n}$ is also an eigenstate of {the symmetrized Hamiltonian} $H+O_g\delta H_{\mr{NH}}O_g^{-1}$. This observation  implies that by averaging $\delta H_{\mr{NH}}$ over the symmetry group,}
\begin{equation}\label{eq:invariant perturbation}
    \delta H^{\mr{inv}}_{\mr{NH}}=\frac{1}{|G|}\sum_{g\in G}O_g\delta H_{\mr{NH}}O_g^{-1}.
\end{equation}
{we obtain a symmetry preserving perturbation $\delta H_{\mr{NH}}^{\mr{inv}}$ with the same exact scar states.}

\subsection{{One-dimensional chain}}
{As discussed in Sec.~\ref{sec:1D perturbation}, $\delta H_{\mr{NH}}$ for the 1D chain is}
\begin{equation}
    {\delta H_{\mr{NH}}=\frac{1}{2}\sum_{b\in\Lambda_{\mr{B}}}P_{2b-1}\left(\sigma^+_{2b}P_{2b+1}+P_{2b}\sigma^+_{2b+1}\right)P_{2b+2}.}
\end{equation}
{The original PXP model on the 1D chain is invariant with respect to translation $T$ by a single $S=1/2$ site, i.e., $[H,T]=0$. The modified $S=1$ model obtained after dimerization is instead symmetric only with respect to translation by two $S=1/2$ sites. From Eq.~\eqref{eq:manifest inv Sn}, however, we see that its scar state $\ket*{S_n}$ is nevertheless invariant under translation, i.e., $T\ket*{S_n}=(-1)^{N-n}\ket*{S_n}$. This indicates that we may average the Hamiltonian over all translations, or equivalently, just  over the two elements $\{id, T\}$ where $id$ is the identity operator. Applying this result to Eq.~\eqref{eq:invariant perturbation}, we obtain}
\begin{equation}
    {\delta H_{\mr{NH}}^{\mr{inv}}=\frac{1}{4}\sum_{i\in\Lambda}P_{i-1}\sigma_i^+P_{i+1}\left(P_{i-2}+P_{i+2}\right).}
\end{equation}

\subsection{{Honeycomb lattice}}
\begin{figure}
    \centering
    \includegraphics[width=.8\textwidth]{honeycomb_perturbation.eps}
    \caption{A graphical representation of rotationally invariant perturbations $\delta H_{\mr{NH}}^{\mr{inv}}$. The black, blue (light grey) and red (grey) dots correspond to the operators $\sigma^+$, $P$, and $1-P$, respectively.}
    \label{fig:honeycomb_perturbation}
\end{figure}
{The non-Hermitian perturbation $\delta H_{\mr{NH}}$ for the honeycomb lattice in Sec.~\ref{sec:honeycomb perturbation} can be written as}
\begin{equation}
    \begin{split}
        {\delta H_{\mr{NH}}}&{=\frac{1}{2}\sum_{\Vec{R}\in\Lambda_{\mr{B}}}\sum_{i=1,2}\left(\ket*{+,0}+\ket*{0,-}\right)\bra*{0,0}_{\Vec{R},\Vec{R}+\Vec{e}_i}-\frac{1}{4}\sum_{\Vec{R}\in\Lambda_{\mr{B}}}\ket*{0,-,-}\left(\bra*{0,0,-}+\bra*{0,-,0}\right)_{\Vec{R},\Vec{R}+\Vec{e}_1,\Vec{R}+\Vec{e}_2}}\\
        &{-\frac{1}{4}\sum_{\Vec{R}\in\Lambda_{\mr{B}}}\ket*{+,+,0}\left(\bra*{0,+,0}+\bra*{+,0,0}\right)_{\Vec{R}-\Vec{e}_1,\Vec{R}-\Vec{e}_2,\Vec{R}}}\\
        &{\equiv\frac{1}{2}\sum_{\Vec{R}\in\Lambda_{\mr{B}}}\sum_{i=1,2}\delta_1h_{\Vec{R},\Vec{R}+\Vec{e}_i}-\frac{1}{4}\sum_{\Vec{R}\in\Lambda_{\mr{B}}}\delta_{2\alpha}h_{\Vec{R},\Vec{R}+\Vec{e}_1,\Vec{R}+\Vec{e}_2}-\frac{1}{4}\sum_{\Vec{R}\in\Lambda_{\mr{B}}}\delta_{2\beta}h_{\Vec{R}-\Vec{e}_1,\Vec{R}-\Vec{e}_2,\Vec{R}}}.
    \end{split}
\end{equation}
{As discussed in the main text, the PXP model on the honeycomb lattice possesses a site-centered rotation symmetry. We denote the corresponding rotation operator by $O_g$, and consider $G=\{id, g, g^2\}$. Applying this to Eq.~\eqref{eq:invariant perturbation}, we obtain the rotationally symmetric perturbation}
\begin{equation}
    {\delta H^{\mr{inv}}_{\mr{NH}}=\frac{1}{6}\sum_{\Vec{r}\in\Lambda_\alpha}\delta_{1\alpha}h^{\mr{inv}}_{\Vec{r}}+\frac{1}{6}\sum_{\Vec{r}\in\Lambda_\beta}\delta_{1\beta}h^{\mr{inv}}_{\Vec{r}}-\frac{1}{12}\sum_{\Vec{r}\in\Lambda_\alpha}\delta_{2\alpha}h^{\mr{inv}}_{\Vec{r}}-\frac{1}{12}\sum_{\vec{r}\in\Lambda_\beta}\delta_{2\beta}h^{\mr{inv}}_{\vec{r}},}
\end{equation}
{where}
\begin{equation}\begin{split}
    {\delta_{1\alpha}h_{\Vec{r}}^{\mr{inv}}}&{=\sum_{g\in G}O_g\left(P_{\Vec{r}+\Vec{e}_y}\sigma^+_{\Vec{r}}P_{\Vec{r}-\Vec{e}_1+\Vec{e}_y}P_{\Vec{r}-\Vec{e}_1}+P_{\vec{r}+\vec{e}_y}\sigma_{\vec{r}}^+P_{\vec{r}-\vec{e}_2+\vec{e}_y}P_{\vec{r}-\vec{e}_2}\right)O_g^{-1}}\\
    {\delta_{1\beta}h_{\Vec{r}}^{\mr{inv}}}&{=\sum_{g\in G}O_g\left(P_{\Vec{r}-\Vec{e}_y}\sigma^+_{\Vec{r}}P_{\Vec{r}+\Vec{e}_1-\Vec{e}_y}P_{\Vec{r}+\Vec{e}_1}+P_{\vec{r}-\vec{e}_y}\sigma^+_{\vec{r}}P_{\vec{r}+\vec{e}_2-\vec{e}_y}P_{\vec{r}+\vec{e}_2}\right)O_g^{-1}}\\ 
    {\delta_{2\alpha}h^{\mr{inv}}_{\Vec{r}}}&{=\sum_{g\in G}O_g\left(P_{\Vec{r}-\Vec{e}_1+\Vec{e}_y}P_{\Vec{r}-\Vec{e}_1}\sigma_{\Vec{r}}^+P_{\Vec{r}+\Vec{e}_y}\left(1-P_{\Vec{r}-\Vec{e}_1+\Vec{e}_2}\right)P_{\Vec{r}-\Vec{e}_1+\Vec{e}_2+\Vec{e}_y}+P_{\Vec{r}-\Vec{e}_1+\Vec{e}_y}P_{\Vec{r}-\Vec{e}_1}\left(1-P_{\Vec{r}}\right)P_{\Vec{r}+\Vec{e}_y}\sigma^+_{\Vec{r}-\Vec{e}_1+\Vec{e}_2}P_{\Vec{r}-\Vec{e}_1+\Vec{e}_2+\Vec{e}_y}\right)O_g^{-1}}\\
    {\delta_{2\beta}h^{\mr{inv}}_{\vec{r}}}&{=\sum_{g\in G}O_g\left(P_{\Vec{r}-\Vec{e}_y}\sigma_{\Vec{r}}^+\left(1-P_{\Vec{r}+\Vec{e}_1-\Vec{e}_2}\right)P_{\Vec{r}+\vec{e}_1-\vec{e}_2-\vec{e}_y}P_{\vec{r}+\vec{e}_1+\vec{e}_y}+P_{\Vec{r}-\Vec{e}_y}\left(1-P_{\Vec{r}}\right)\sigma^+_{\Vec{r}+\Vec{e}_1-\Vec{e}_2}P_{\Vec{r}+\vec{e}_1-\vec{e}_2-\vec{e}_y}P_{\vec{r}+\vec{e}_1+\vec{e}_y}\right)O_g^{-1}.}
    \end{split}
\end{equation}
{Fig.~\ref{fig:honeycomb_perturbation} illustrates the above operators graphically.}

\section{Alternative derivation of known exact eigenstates of the PXP model}\label{app:ML state}
There are several exact eigenstates known for the PXP model~\cite{Lin2019mps}: one specific zero-energy eigenstate for PBC, and four eigenstates for open boundary condition (OBC). Their wavefunctions were originally expressd as matrix product states (MPS), and it was pointed out that a basis transformation connects the zero energy eigenstate to the ground state of the AKLT model. Later, Ref.~\cite{Shiraishi_2019} gave an elegant proof of that state being a zero energy eigenstate, by showing that the basis transformation yields {the projector-embedding} form $H=\sum_i\mc{P}_ih_i\mc{P}_i+H'$ where $\mc{P}_i$ is a local projection operator that annihilates the AKLT ground state, and so does $H'$. %This form of the Hamiltonian enables a so-called projector embedding of scar states, which allows for a systematic construction of ETH-violating models~\cite{mori_shiraishi}.   

In this section, we give an alternative  proof of these exact eigenstates based on the block spin representation introduced in the main text.
\subsection{Enlarging the Hilbert space}%Fractionalization}
%\MM{this is exactly the same mapping as discussed in the main text. So we should refer to it. I would say that it identifies a subspace of the s=1/2 model with the S=1 block spins. Reading it in the reverse sense, it embeds the S=1 model into a larger space, whereby the S=1 spins are re-fractionalized. But it seems a bit artificial to call the undoing of spin blocking a fractionalization. At least we should explain a bit more about hat we have in mind here.}

%\MM{I would think this should go into a separate paper, no? Or, if you want to keep it, you have to explain here what is the ultimate goal of this appendix.}
%As mentioned in the main text, the AKLT model can be decomposed as $H_{\mr{spec}}+H_{\mr{ann}}$ and the latter term is a sum of local operators only in an enlarged Hilbert space.
{In order to show that the states introduced in Ref.~\cite{Lin2019mps} are eigenstates, ``fractional" spins representation of the $S=1$ element play a vital role.} Here we introduce a map which identifies a subspace of the $S=1/2$ model with the $S=1$ block spin~\cite{Tasaki2020}:
%In order to do so, we introduce a notion of fractionalizing the $N$ $S=1$ units into $2N$ $S=1/2$ elements~\cite{Tasaki2020}. 
%We define a map $A_b:\mb{C}^{2\otimes2}\rightarrow\mb{C}^3$ for $\forall b\in\Lambda_{\mr{B}}$:
\begin{equation}
    A_b\coloneqq\ket*{+}_b\bra*{\uparrow\uparrow}_{(b,\mr{L}),(b,\mr{R})}+\ket*{0}_b\frac{1}{\sqrt{2}}\left(\bra*{\uparrow\downarrow}+\bra*{\downarrow\uparrow}\right)_{(b,\mr{L}),(b,\mr{R})}+\ket*{-}_b\bra*{\downarrow\downarrow}_{(b,\mr{L}),(b,\mr{R})},
\end{equation}
where $(b,\mr{L/R})\in\Lambda_{\mr{B}}^{\mr{frac}}\coloneqq\Lambda_{\mr{B}}\times\{\mr{L},\mr{R}\}$ labels the lattice sites for ``fractional" $S=1/2$ elements. %Physical meaning of this map is to regard one particle with spin-$1$ as a composite state of two particles with spin-$1/2$, which can be done by discarding the singlet component. 
We also define the natural tensor product of this map over blocks as $\msf{A}\coloneqq\prod_{b\in\Lambda_{\mr{B}}}A_b:\mb{C}^{2\otimes2\otimes N}\rightarrow\mb{C}^{3\otimes N}$.  

We can fractionalize the spin operator as well. For an arbitrary operator $O:\mb{C}^{3\otimes N}\rightarrow\mb{C}^{3\otimes N}$ of $S=1$ units, there exists an operator $O_{\mr{frac}}:\mb{C}^{2\otimes2\otimes N}\rightarrow\mb{C}^{2\otimes2\otimes N}$ such that $O\msf{A}=\msf{A}O_{\mr{frac}}$. Obviously the choice of $O_{\mr{frac}}$ is not unique. For example, both operators $\sqrt{2}\dyad*{\uparrow\uparrow}{\uparrow\downarrow}_{(b,\mr{L}),(b,\mr{R})}$ and $\sqrt{2}\dyad*{\uparrow\uparrow}{\downarrow\uparrow}_{(b,\mr{L}),(b,\mr{R})}$ correspond to $\dyad*{+}{0}$. However, there is a natural choice for $O_{\mr{frac}}$: we first note that for any operator-valued function $F$, it holds that
\begin{equation}\label{eq:operator identity}
    F(\{\bm{S}_b\}_{b\in\Lambda_{\mr{B}}})\msf{A}=\msf{A}F\left(\left\{\bm{S}_{(b,\mr{L})}+\bm{S}_{(b,\mr{R})}\right\}_{b\in\Lambda_{\mr{B}}}\right),
\end{equation}
where $\bm{S}_b$ is a spin operator with $S=1$, i.e., $\bm{S}_b:\mb{C}^3\rightarrow\mb{C}^3$, and $\bm{S}_{(b,\mr{L/R})}$ is a spin operator with $S=1/2$, i.e., $\bm{S}_{(b,\mr{L/R})}:\mb{C}^2\rightarrow\mb{C}^2$. %This is physically quite natural, as the spin operator $\bm{S}_b$ is split into a sum of two spin operators $\bm{S}_{(b,\mr{L})}+\bm{S}_{(b,\mr{R})}$.
\subsection{Defining exact eigenstates}
%\MM{We will show that the following states are eigenstates ...? instead of: } 
We will show that the following states $\ket*{\Gamma}$ and $\ket*{\Gamma^{\tau\tau'}}$ are eigenstates of the unperturbed PXP model with PBC and with OBC, respectively:%We consider the following states as candidates for a zero energy eigenstate $\ket*{\Gamma}$ with PBC and for four eigenstates $\ket*{\Gamma^{\tau\tau'}}$ with OBC:
\begin{equation}\label{eq:|Gamma> in SM}
    \begin{split}
        \ket*{\Gamma}&=\msf{A}\bigotimes_{b\in\Lambda_{\mr{B}}}\frac{1}{\sqrt{2}}\left(\ket*{\uparrow\uparrow}-\ket*{\downarrow\downarrow}\right)_{(b,\mr{R}),(b+1,\mr{L})}\\
        \ket*{\Gamma^{\tau\tau'}}&=\msf{A}\bigotimes_{b\in\Lambda_{\mr{B}}\setminus\{N\}}\frac{1}{\sqrt{2}}\left(\ket*{\uparrow\uparrow}-\ket*{\downarrow\downarrow}\right)_{(b,\mr{R}),(b+1,\mr{L})}\otimes\ket*{\tau}_{(1,\mr{L})}\ket*{\tau'}_{(N,\mr{R})},
    \end{split}
\end{equation}
where $\ket*{\tau}$ and $\ket*{\tau'}$ are either $\ket*{\rightarrow}\coloneqq(\ket*{\uparrow}+\ket*{\downarrow})/\sqrt{2}$ or $\ket*{\leftarrow}\coloneqq(\ket*{\uparrow}-\ket*{\downarrow})/\sqrt{2}$, namely eigenstates of $X(\equiv\dyad*{\uparrow}{\downarrow}+\dyad*{\downarrow}{\uparrow})$. %\MM{have you defined X and Z?}. 
Pictorial representations of these states are shown in Fig.~\ref{fig:VBS}. Note the great similarity of the diagrams in Fig.~\ref{fig:VBS} with depictions of the AKLT ground state. 
\begin{figure}
    \centering
    \includegraphics[width=.65\textwidth]{valence_bond_solid.eps}
    \caption{Pictorial representations of $\ket*{\Gamma}$ and $\ket*{\Gamma^{\rightarrow\rightarrow}}$. A line corresponds to the triplet state $(\ket*{\uparrow\uparrow}-\ket*{\downarrow\downarrow})/\sqrt{2}$, while  an oval indicates the symmetrization $\msf{A}$.}
    \label{fig:VBS}
\end{figure}

We first show that these states belong to $\mc{V}_{\mr{Ryd}}$. To do so, we consider the following 2-block states:
\begin{equation}
    \ket*{\gamma^{\sigma\sigma'}_{b,b+1}}\coloneqq \ket{\sigma}_{(b,\mr{L})}\frac{1}{\sqrt{2}}\left(\ket{\uparrow\uparrow}-\ket{\downarrow\downarrow}\right)_{(b,\mr{R}),(b+1,\mr{L})}\ket*{\sigma'}_{b+1,\mr{R}},
\end{equation}
where $\sigma$ and $\sigma'$ are either $\uparrow$ or $\downarrow$, that is, eigenstates of  $Z$. The states $\ket*{\Gamma}$ and $\ket*{\Gamma^{\tau\tau'}}$ can now be expressed in terms  of these $\ket*{\gamma^{\sigma\sigma'}_{b,b+1}}$ as:% in the sense that for $\forall b\in\Lambda_{\mr{B}}$, one can express them as 
\begin{equation}\label{eq:|Gamma> decomposition}
    \begin{split}
         \ket*{\Gamma}&=\msf{A}\sum_{\sigma,\sigma'=\uparrow,\downarrow}c_{\sigma\sigma'}\ket*{\gamma^{\sigma\sigma'}_{b,b+1}}\otimes\ket*{\Xi_{\sigma\sigma'}}\\
         \ket*{\Gamma^{\tau\tau'}}&=\msf{A}\sum_{\sigma,\sigma'=\uparrow,\downarrow}c_{\sigma\sigma'}\ket*{\gamma^{\sigma\sigma'}_{b,b+1}}\otimes\ket*{\Xi^{\tau\tau'}_{\sigma\sigma'}},
    \end{split}
\end{equation}
where $c_{\sigma\sigma'}$ are coefficients and $\ket*{\Xi_{\sigma\sigma'}}$ and $\ket*{\Xi_{\sigma\sigma'}^{\tau\tau'}}$ are spin-$1/2$ wavefunctions defined on $(\Lambda_{\mr{B}}\setminus\{b,b+1\})\times\{\mr{L},\mr{R}\}$.
A straightforward calculation yields
\begin{equation}
    \begin{split}
        A_b\otimes A_{b+1}\ket*{\gamma_{b,b+1}^{\uparrow\uparrow}}&=\frac{1}{\sqrt{2}}\ket*{+,+}_{b,b+1}-\frac{1}{2\sqrt{2}}\ket*{0,0}_{b,b+1}\\
        A_b\otimes A_{b+1}\ket*{\gamma_{b,b+1}^{\uparrow\downarrow}}&=\frac{1}{2}\ket*{+,0}_{b,b+1}-\frac{1}{2}\ket*{0,-}_{b,b+1}\\
        A_b\otimes A_{b+1}\ket*{\gamma_{b,b+1}^{\downarrow\uparrow}}&=\frac{1}{2}\ket*{0,+}_{b,b+1}-\frac{1}{2}\ket*{-,0}_{b,b+1}\\
        A_b\otimes A_{b+1}\ket*{\gamma_{b,b+1}^{\downarrow\downarrow}}&=\frac{1}{2\sqrt{2}}\ket*{0,0}_{b,b+1}-\frac{1}{\sqrt{2}}\ket*{-,-}_{b,b+1}.
    \end{split}
\end{equation}
Therefore, combined with Eq.~\eqref{eq:|Gamma> decomposition}, one finds 
\begin{equation}\label{eq:local Pryd}
    \begin{split}
        (1-\dyad{+,-})_{b,b+1}\ket*{\Gamma}&=+\ket*{\Gamma}\\
        (1-\dyad{+,-})_{b,b+1}\ket*{\Gamma^{\tau\tau'}}&=+\ket*{\Gamma^{\tau\tau'}}
    \end{split}
\end{equation}
for $\forall b\in\Lambda_{\mr{B}}$. Since $P_{\mr{Ryd}}$ is the product over $b$ of $\left(1-\dyad{+,-}\right)_{b,b+1}$ and %$\left[(1-\dyad{+,-})_{b,b+1},(1-\dyad{+,-})_{b',b'+1}\right]=0$ for $\forall b,b'\in\Lambda_{\mr{B}}$, namely 
and local Rydberg constraints ($1-\dyad*{+,-}_{b,b+1}$) commute with each other, we find $P_{\mr{Ryd}}\ket*{\Gamma}=+\ket*{\Gamma}$ and $P_{\mr{Ryd}}\ket*{\Gamma^{\tau\tau'}}=+\ket*{\Gamma^{\tau\tau'}}$, implying $\ket*{\Gamma},\ket*{\Gamma^{\tau\tau'}}\in\mc{V}_{\mr{Ryd}}$.

\subsection{A detailed proof of the  eigenstate property}
As $P_{\mr{Ryd}}\ket*{\Gamma}=+\ket*{\Gamma}$, it holds that
\begin{equation}
    H\ket*{\Gamma}=HP_{\mr{Ryd}}\ket*{\Gamma}=P_{\mr{Ryd}}H\ket*{\Gamma}=P_{\mr{Ryd}}\left(H_{\mr{Z}}+H_1\right)\ket*{\Gamma}.
\end{equation}
Here we use $\left[P_{\mr{Ryd}},H\right]=0$ and $P_{\mr{Ryd}}\ket*{+,-}=0$. Further, Eq.~\eqref{eq:local Pryd} implies that $\dyad*{+,-}_{b,b+1}\ket*{\Gamma}=0$ for $\forall b\in\Lambda_{\mr{B}}$, and thus $H_1 \ket*{\Gamma}=0$.
We therefore obtain $H\ket*{\Gamma}=P_{\mr{Ryd}}H_{\mr{Z}}\ket*{\Gamma}$.
The same relation holds for $\ket*{\Gamma^{\tau\tau'}}$ as well. With the operator identity of Eq.~\eqref{eq:operator identity}, we find 
\begin{equation}\begin{split}
    H_{\mr{Z}}\ket{\Gamma}&=\msf{A}\left(\sqrt{2}\sum_{b\in\Lambda_{\mr{B}}}\left(\frac{1}{2}X_{(b,\mr{L})}+\frac{1}{2}X_{(b,\mr{R})}\right)\right)\bigotimes_{b'\in\Lambda_{\mr{B}}}\frac{1}{\sqrt{2}}\left(\ket{\uparrow\uparrow}-\ket{\downarrow\downarrow}\right)_{(b',\mr{R}),(b'+1,\mr{L})}\\
    &=\msf{A}\left(\sqrt{2}\sum_{b\in\Lambda_{\mr{B}}}\left(\frac{1}{2}X_{(b,\mr{R})}+\frac{1}{2}X_{(b+1,\mr{L})}\right)\right)\bigotimes_{b'\in\Lambda_{\mr{B}}}\frac{1}{\sqrt{2}}\left(\ket{\uparrow\uparrow}-\ket{\downarrow\downarrow}\right)_{(b',\mr{R}),(b'+1,\mr{L})}\\&=0,
    \end{split}
\end{equation}
where the PBC was used in the second line. For $\ket*{\Gamma^{\tau\tau'}}$, we find
\begin{equation}
    \begin{split}
        H_{\mr{Z}}\ket*{\Gamma^{\tau\tau'}}&=\msf{A}\left(\sqrt{2}\sum_{b\in\Lambda_{\mr{B}}}\left(\frac{1}{2}X_{(b,\mr{L})}+\frac{1}{2}X_{(b,\mr{R})}\right)\right)\bigotimes_{b'\in\Lambda_{\mr{B}}\setminus\{N\}}\frac{1}{\sqrt{2}}\left(\ket*{\uparrow\uparrow}-\ket*{\downarrow\downarrow}\right)_{(b',\mr{R}),(b'+1,\mr{L})}\otimes\ket*{\tau}_{(1,\mr{L})}\ket*{\tau'}_{(N,\mr{R})}\\
        &=\msf{A}\frac{1}{\sqrt{2}}\left(X_{(1,\mr{L})}+X_{(N,\mr{R})}\right)\bigotimes_{b'\in\Lambda_{\mr{B}}\setminus\{N\}}\frac{1}{\sqrt{2}}\left(\ket*{\uparrow\uparrow}-\ket*{\downarrow\downarrow}\right)_{(b',\mr{R}),(b'+1,\mr{L})}\otimes\ket*{\tau}_{(1,\mr{L})}\ket*{\tau'}_{(N,\mr{R})}.
    \end{split}
\end{equation}
Since $\ket{\tau}$ and $\ket*{\tau'}$ were chosen as eigenstates of $X$, $\ket*{\Gamma^{\tau\tau'}}$ is seen to be an eigenstate of $H_{\mr{Z}}$.

\subsection{Matrix product state (MPS)  representation}
In Ref.~\cite{Lin2019mps}, $\ket*{\Gamma}$ and $\ket*{\Gamma^{\tau\tau'}}$ were given as MPS. Here we re-derive their MPS representation. % and show an equivalence between the states considered in Ref.~\cite{Lin2019mps} and the states in Eq.~\eqref{eq:|Gamma> in SM}. 
To do so, we define a bond variable $\rket{\alpha}_b$ %:\{1,2\}\rightarrow\{\ket*{\uparrow\uparrow}_{(b-1,\mr{R}),(b,\mr{L})},\ket*{\downarrow\downarrow}_{(b-1,\mr{R}),(b,\mr{L})}\}$
for $b\in\Lambda_{\mr{B}}$ such that
\begin{equation}
    \rket{0}_b\coloneqq\ket*{\uparrow\uparrow}_{(b-1,\mr{R}),(b,\mr{L})},\,\,
    \rket{1}_b\coloneqq\ket*{\downarrow\downarrow}_{(b-1,\mr{R}),(b,\mr{L})}.
\end{equation}
$\ket*{\Gamma}$ is re-written as
\begin{equation}
    \begin{split}
        \ket*{\Gamma}&=\msf{A}\bigotimes_{b\in\Lambda_{\mr{B}}}\frac{1}{\sqrt{2}}\left(\rket{0}-\rket{1}\right)_b.
    \end{split}
\end{equation}
From this expression, we can find the MPS representation for $\ket*{\Gamma}$: a straightforward calculation yields %\MM{Notation $| 0>^b$ means $| 0>_b$ and is different from $|0)_b$, right? You should point out that it is different.}
\begin{equation}\label{eq:Ab}\begin{split}
    A_b\frac{1}{\sqrt{2}}\left(\rket{0}-\rket{1}\right)_b\otimes\frac{1}{\sqrt{2}}\left(\rket{0}-\rket{1}\right)_{b+1}&=\msf{A}_{1,1}^+\ket*{\uparrow}_{(b-1,\mr{R})}\ket*{+}_b\ket*{\uparrow}_{(b+1,\mr{L})}+\msf{A}_{1,2}^0\ket*{\uparrow}_{(b-1,\mr{R})}\ket*{0}_b\ket*{\downarrow}_{(b+1,\mr{L})}\\
    &-\msf{A}_{2,1}^0\ket*{\downarrow}_{(b-1,\mr{R})}\ket*{0}_b\ket*{\uparrow}_{(b+1,\mr{L})}-\msf{A}_{2,2}^-\ket*{\downarrow}_{(b-1,\mr{R})}\ket*{-}_b\ket*{\downarrow}_{(b+1,\mr{L})},
    \end{split}
\end{equation}
where 
\begin{equation}
\msf{A}_{1,1}^+\coloneqq\frac{1}{2},\,\,\msf{A}^0_{1,2}\coloneqq-\frac{1}{2\sqrt{2}},\,\,\msf{A}^0_{2,1}\coloneqq\frac{1}{2\sqrt{2}},\,\,\msf{A}^-_{2,2}\coloneqq-\frac{1}{2}.
\end{equation}
We emphasize that $\rket{0}_b$ is different from $\ket*{0}_b$ in Eq.~\eqref{eq:Ab}: $\rket{0}_b$ is a bond variable and $\ket*{0}_b$ is an eigenstate of $S^z_b$.
$\ket*{\Gamma}$ can be written as
\begin{equation}
    \ket*{\Gamma}=\sum_{\{\sigma_i\}_{i=1}^N\in\{\pm,0\}^{\otimes N}}\mr{Tr}\left[\msf{A}^{\sigma_1}\cdots\msf{A}^{\sigma_{N}}\right]\ket*{\sigma_1\cdots\sigma_N},
\end{equation}
where 
\begin{equation}
    \msf{A}^+\coloneqq\frac{1}{2\sqrt{2}}\begin{pmatrix}\sqrt{2} & 0\\0&0\end{pmatrix},\,\,\msf{A}^0\coloneqq\frac{1}{2\sqrt{2}}\begin{pmatrix}0&-1\\1&0\end{pmatrix},\,\,\msf{A}^-\coloneqq\frac{1}{2\sqrt{2}}\begin{pmatrix}0&0\\0&-\sqrt{2}\end{pmatrix}.
\end{equation}
Up to an irrelevant normalization factor, this is the same as the zero energy state given in Ref.~\cite{Lin2019mps}.

A similar calculation leads to the MPS representation of $\ket*{\Gamma^{\tau\tau'}}$:
\begin{equation}
    \begin{split}
        \ket*{\Gamma^{\tau\tau}}=\sum_{\{\sigma_i\}_{i=1}^N\in\{\pm,0\}^{\otimes N}}\left(\msf{v}_\tau^{\sigma_1}\right)^{\mr{T}}\msf{A}^{\sigma_2}\cdots\msf{A}^{\sigma_{N-1}}\msf{w}_{\tau'}^{\sigma_N}\ket*{\sigma_1\cdots\sigma_N},
    \end{split}
\end{equation}
where 
\begin{equation}
    \begin{split}
        \msf{v}_\rightarrow^+&\coloneqq\frac{1}{2}\begin{pmatrix}\sqrt{2}\\0\end{pmatrix},\,\,\msf{v}_\rightarrow^0\coloneqq\frac{1}{2}\begin{pmatrix}1\\-1\end{pmatrix},\,\,\msf{v}_\rightarrow^-\coloneqq\frac{1}{2}\begin{pmatrix}0\\-\sqrt{2}\end{pmatrix},\,\,\msf{v}^+_\leftarrow\coloneqq\frac{1}{2}\begin{pmatrix}\sqrt{2}\\0\end{pmatrix},\,\,\msf{v}^0_\leftarrow\coloneqq\frac{1}{2}\begin{pmatrix}-1\\-1\end{pmatrix},\,\,\msf{v}_\leftarrow^-\coloneqq\frac{1}{2}\begin{pmatrix}0\\\sqrt{2}\end{pmatrix},\\
        \msf{w}_\rightarrow^+&\coloneqq\frac{1}{2\sqrt{2}}\begin{pmatrix}\sqrt{2}\\0\end{pmatrix},\,\,\msf{w}_\rightarrow^0\coloneqq\frac{1}{2\sqrt{2}}\begin{pmatrix}1\\1\end{pmatrix},\,\,\msf{w}_\rightarrow^-\coloneqq\frac{1}{2\sqrt{2}}\begin{pmatrix}0\\\sqrt{2}\end{pmatrix},\,\,\msf{w}_\leftarrow^+\coloneqq\frac{1}{2\sqrt{2}}\begin{pmatrix}\sqrt{2}\\0\end{pmatrix},\,\,\msf{w}_\leftarrow^0\coloneqq\frac{1}{2\sqrt{2}}\begin{pmatrix}-1\\1\end{pmatrix},\,\,\msf{w}_\leftarrow^-\coloneqq\frac{1}{2\sqrt{2}}\begin{pmatrix}0\\-\sqrt{2}\end{pmatrix}.
    \end{split}
\end{equation}
The relations
\begin{equation}\begin{split}
\begin{pmatrix}1&1\end{pmatrix}\msf{A}^\sigma&=\frac{1}{\sqrt{2}}\msf{v}^\sigma_\rightarrow,\,\,\begin{pmatrix}1&-1\end{pmatrix}\msf{A}^\sigma=\frac{1}{\sqrt{2}}\msf{v}^\sigma_\leftarrow,\,\,\msf{A}^\sigma\begin{pmatrix}1\\1\end{pmatrix}=\msf{w}^\sigma_\leftarrow,\,\,\msf{A}^\sigma\begin{pmatrix}1\\-1\end{pmatrix}=\msf{w}^\sigma_\rightarrow,
\end{split}
\end{equation}
finally establish the equivalence of the states $\ket*{\Gamma^{\tau\tau}}$
to the four eigenstates given in Ref.~\cite{Lin2019mps}.
%Note that we have
%\begin{equation}\begin{split}
    %A_b\rket{1,1}_{b,b+1}&=\ket*{\uparrow}_{(b-1,\mr{R})}\ket*{+}_b\ket*{\uparrow}_{(b+1,\mr{L})},\,\,A_b\rket{1,2}_{b,b+1}=\ket*{\uparrow}_{(b-1,\mr{R})}\frac{1}{\sqrt{2}}\ket*{0}_b\ket*{\downarrow}_{(b+1,\mr{L})}\\
    %A_b\rket{2,1}_{b,b+1}&=\ket*{\downarrow}_{(b-1,\mr{R})}\frac{1}{\sqrt{2}}\ket*{0}_b\ket*{\uparrow}_{(b+1,\mr{L})},\,\,A_b\rket{2,2}_{b,b+1}=\ket*{\downarrow}_{(b-1,\mr{R})}\ket*{-}_b\ket*{\downarrow}_{(b+1,\mr{L})}.
    %\end{split}
%\end{equation}
%an operator $B:\{1,2\}\times\{1,2\}\rightarrow\mb{C}^3$ such that
%\begin{equation}
    %B(1,1)=A_b
%\end{equation}
\subsection{Alternative set of trial wave functions}
In the main text, we consider the trial wave functions $\ket*{S_n}$, which are viewed as projections on ${\cal V}_{\rm Ryd}$ of the eigenstates of $H_{\mr{Z}}$ with maximal total pseudospin. However, one can also construct an alternative set of trial wave functions based on the exact reference scar state $\ket*{\Gamma}$. We consider the ansatz
\begin{equation}\label{eq:another Sn}
    \ket*{\mr{MPS}_n}\coloneqq P_{\mr{Ryd}}\left(J^+\right)^n\ket*{\Gamma},
\end{equation}
where $J^\pm$ is defined in %\MM{Eq.~(XXX) of} 
the main text. In the spin-$1/2$ representation, $\ket*{\mr{MPS}_n}$ is expressed as 
\begin{equation}\label{eq:|MPS>}
    \begin{split}
        \ket*{\mr{MPS}_n}&=\sum_{\{b_k\}_{k=1}^n\subset\Lambda_{\mr{B}}}P_{\mr{Ryd}}\msf{A}\bigotimes_{k=1}^n\ket*{\rightarrow\rightarrow}_{(b_k,\mr{R}),(b_k+1,\mr{L})}\bigotimes_{b'\in\Lambda_{\mr{B}}\setminus\{b_k\}_{k=1}^n}\frac{1}{\sqrt{2}}\left(\ket*{\uparrow\uparrow}-\ket*{\downarrow\downarrow}\right)_{(b',\mr{R}),(b'+1,\mr{L})}.
    \end{split}
\end{equation}

We numerically find that these states have similarly high overlap with the exact scar states as $\ket*{S_n}$, cf. Fig.~\ref{fig:overlap_MPs}. We note, however, that they become increasingly worse approximations once scar-enhancing perturbations are added to the Hamiltonian.%, as is shown in  Fig.~\ref{fig:overlap_MPs}.%However, it is expected that they yield a better estimate for the energies of scar states having small energy, i.e., small index $n$.% squared overlap $|\innerproduct*{\mr{MPS}_n}{\mc{S}^{\mr{PXP}}_n}|^2$ is roughly as large as $|\innerproduct*{S_n}{\mc{S}^{\mr{PXP}}_n}|^2$ as shown in Fig.~\ref{fig:overlap_MPs}. 
\begin{figure}
    \centering
    \includegraphics[width=.6\textwidth]{overlap_MPs.eps}
    \caption{Square of the overlap $|\innerproduct*{\mc{S}_n^{\mr{PXP}}}{\mr{MPS}_n}|^2$ between the exact scar states $\ket*{\mc{S}_n^{\mr{PXP}}}$ and the trial wave functions $\ket*{\mr{MPS}_n}$ from Eq.~(\ref{MPS}).}
    \label{fig:overlap_MPs}
\end{figure}

\section{Energy of the trial scar states}
In this appendix we estimate the energy of the scar states in the tail of the spectrum, i.e., for $\ket*{\mc{S}^{\mr{PXP}}_{N_b}}$ and $\ket*{\mc{S}^{\mr{PXP}}_{N_b-1}}$, as well as in the middle of the spectrum (for $\ket*{\mc{S}^{\mr{PXP}}_1}$), by evaluating the expectation value of $H$ on our approximate trial wavefunctions.
{Here we restrict ourselves to the 1D chain, but the generalization to any lattice, including the honeycomb lattice discussed in the main text, is straightforward.}
\subsection{{Energy estimate using $\ket*{S_n}$}}\label{app:energy general}
{Here we estimate the energy of the scar states using our ansatz $\ket*{S_n}$, based on first-order perturbation theory. As discussed in the main text, one finds}
\begin{equation}
\begin{split}
    H\ket*{S_n}&=P_{\mr{Ryd}}\left(H_{\mr{Z}}+H_1+H_2\right)\ket*{\wtil{S}_n}\\&=P_{\mr{Ryd}}\left(H_{\mr{Z}}+H_1\right)\ket*{\wtil{S}_n}
    \label{eq:perturbation}\\&=n\sqrt{2}\ket*{S_n}+P_{\mr{Ryd}}H_1\ket*{\wtil{S}_n},
    \end{split}
\end{equation}
where $\ket*{\wtil{S}_n}$ is an (unnormalized) eigenstate of the Zeeman term with eigenvalue $n\sqrt{2}$. 
To derive an energy correction, we do not directly compute the expectation value of $H$ in the ansatz state $\ket*{S_n}$. Instead we consider the second line of Eq.~\eqref{eq:perturbation} and observe that $\ket*{\wtil{S}_n}$ is an eigenstate  of the Zeeman term $H_Z$ 
within the spin-1 space. We then 
ask  by how much $H_1$ shifts the corresponding eigenvalue within first porder perturbation theory. This is expected to give a good estimate of the energy shift for $\ket*{S_n}$ as well, but allows us to circumvent the difficulties related to the Rydberg constraint.
  We thus regard $H_{\mr{Z}}$ and $\ket*{\wtil{S}_n}$ as the unperturbed Hamiltonian, and the unperturbed states, respectively, and $H_1$ as a (non-Hermitian) perturbation. The first order energy correction is given as
\begin{equation}\label{eq:perturbation2}
    \begin{split}
        {\Delta E_n=\frac{\expval*{H_1}{\wtil{S}_n}}{\mc{N}_n} =\frac{1}{\mc{N}_n}\sum_b\bra*{\wtil{S}_n}\left(\ket*{+,0}+\ket*{0,-}\right)\bra*{+,-}_{b,b+1}\ket*{\wtil{S}_n},}
    \end{split}
\end{equation}
{where $\mc{N}_n=\innerproduct*{\wtil{S}_n}$ is the norm of the (non-normalized) parent scar wavefunction. %Note that $\ket*{\wtil{S}_n}$ is not normalized. 
We now compute the correction from each local term ($(\ket*{+,-}+\ket*{0,-})\bra*{+,-}$). To do so, we first re-write the ansatz $\ket*{\wtil{S}_n}$ for the $n$'th scar state in a suitable way,} %\MM{I think it was misleading to write $S_n$ here, we should only write unprojected wavefunctions.}
\begin{equation}\begin{split}
    %{\ket{S_n}}{=P_{\mr{Ryd}}
   \ket*{\wtil{S}_n}&=
    %P_{\mr{Ryd}}
    \left(J^-\right)^{N-n}\bigotimes_{b\in\Lambda_{\mr{B}}}\ket*{\what{+}}_b,
    \\
    J^\pm&=\sqrt{2}\sum_{b\in\Lambda_{\mr{B}}}\left(\dyad*{\what{\pm}}{\what{0}}+\dyad*{\what{0}}{\what{\mp}}\right)_b.
    \end{split}
\end{equation}
{We split the collective spin-raising (lowering) operator as}
\begin{equation}\begin{split}
    {J^\pm}&{=J_{b,b+1}^\pm+J_{\Lambda_{\mr{B}}\setminus\{b,b+1\}}^\pm},\\
    {J_{b,b+1}^\pm}&{\coloneqq\sqrt{2}\left(\dyad*{\what{\pm}}{\what{0}}+\dyad*{\what{0}}{\what{\mp}}\right)_b+\sqrt{2}\left(\dyad*{\what{\mp}}{\what{0}}+\dyad*{\what{0}}{\what{\mp}}\right)_{b+1}},\\
    {J^\pm_{\Lambda_{\mr{B}}\setminus\{b,b+1\}}}&{\coloneqq\sqrt{2}\sum_{b'\in\Lambda_{\mr{B}}\setminus\{b,b+1\}}\left(\dyad*{\what{\pm}}{\what{0}}+\dyad*{\what{0}}{\what{\mp}}\right)_{b'}.}
    \end{split}
\end{equation}
{Using these operators, we can write $\ket*{\wtil{S}_{N-n}}$ as}
\begin{equation}\label{eq:|Sn> split}\begin{split}
    {\ket*{\wtil{S}_{N-n}}}&{=\sum_{k=0}^{\min\{n,4\}}\binom{n}{k}\left(J^-_{b,b+1}\right)^k\ket*{\what{T}_{2,2}}_{b,b+1}\otimes\left(J^-_{\Lambda_{\mr{B}}\setminus\{b,b+1\}}\right)^{n-k}\ket*{\what{T}_{N-2,N-2}}_{\Lambda_{\mr{B}}\setminus\{b,b+1\}}}\\
    &{=\sum_{m=\max\{2-n,-2\}}^2c_m\ket*{\what{T}_{2,m}}_{b,b+1}\otimes\ket*{\what{T}_{N-2,N-n-m}}_{\Lambda_{\mr{B}}\setminus\{b,b+1\}},}
    \end{split}
\end{equation}
where $c_m$ are numerical constants and $\ket*{\what{T}_{S,M}}$ is a state with total spin $S$ and $S^x=M$. Below we will mostly need the coefficients $c_{\pm2}$ for $n\geq4$, which take the values
\begin{eqnarray}
\label{c2_1}
    c_{2}&=&\prod_{M=N_b-n-1}^{N_b-2}\sqrt{(N_b-2)(N_b-1)-M(M-1)},\\c_{-2}&=&n(n-1)(n-2)(n-3)\prod_{M=N_b-n+3}^{N_b-2}\sqrt{(N_b-2)(N_b-1)-M(M-1)}.\nonumber
\end{eqnarray}
{The matrix element of a local term of $H_1$, which we denote by $\delta e^m_b$, is obtained as}
\begin{equation}
    {\delta e^m_b\coloneqq-\bra*{\what{T}_{2,m}}\left(\ket*{+,0}+\ket*{0,-}\right)\braket*{+,-}{\what{T}_{2,m}}=}\begin{dcases}
    -\frac{\sqrt{2}}{8}&\,\,m=+2,\\
    +\frac{\sqrt{2}}{8}&\,\,m=-2,\\
    0&\,\,\mr{else}.
    \end{dcases}
\end{equation}
{The energy correction from all the sites is thus estimated as,} 
\begin{equation}
\label{eq:energy correction formula}
    {\Delta E_{N_b-n}=\sum_{b\in\Lambda_{\mr{B}}}\sum_{m=-2}^2\delta e^m_b\frac{|c_m|^2}{\mc{N}_{N_b-n}}=-\frac{\sqrt{2}}{8}N_b\frac{|c_2|^2-|c_{-2}|^2}{\mc{N}_{N_b-n}}.}
\end{equation}
{From the elementary theory of angular momentum, the norm $\mc{N}_{N_b-n}$ is easily calculated,}
\begin{equation}
\label{norm}
    {\mc{N}_{N_b-n}=\prod_{M=N_b-n+1}^{N_b}\left(N_b(N_b+1)-M(M-1)\right).}
\end{equation}
%{Note that from Eq.~\eqref{eq:|Sn> split} and Eq.~\eqref{eq:energy correction formula} \MM{why D5 and D7? it seems one should look at D7 and D8?} one finds that for the 1D case absolute value of the energy correction $\Delta E_n$ monotonically increases with increasing $n$ since $|c_{-2}|$ decreases as $n$ increases, while $|c_2|$ increases. \MM{since you don't give formulae for the c's here this cannot be understood. Either shift this statement, to where it can be understod or drop it.}}

\subsubsection{{The tail of the scar spectrum}}\label{app:energy tail}
{The estimate of $E_{N_b}$ and $E_{N_b-1}$ is relatively straightforward. Indeed, for {$n=0$}, one immediately finds $|c_2|^2=\mc{N}_{N_b}$ and $c_{-2}=0$. Therefore the energy correction becomes $\Delta E_{N_b}=-\sqrt{2}/8\times N_b$. Thus, the energy of the state $\ket*{S_n}$ is estimated as $E_{N_b}=7\sqrt{2}N_b/8$. 
For $N_b=10$, our estimate yields $E_{N_b}=70\sqrt{2}/8\approx12.37$, which is within 3 percent of the numerically determined eigenvalue of the exact scar state, $E_{N_b}\approx12.07$. 

For {$n=1$}, a straightforward calculation yields $|c_2|^2/\mc{N}_{N_b-1}=(N_b-2)/N_b$, {and also here $c_{-2}=0$}, which implies $\Delta E_{N_b-1}=-\sqrt{2}/8\times(N_b-2)$. Thus, we obtain the estimate $E_{N_b-1}=(7N_b-6)\sqrt{2}/8$. For $N_b=10$, this yields $11.37$, which is close to the numerical value $E_{N_b-1}\approx11.10$. {The energy spacing in the tails of the spectrum can thus be estimated as $\Delta E_{\mr{tail}}=E_{N_b}-E_{N_b-1}\approx(3/4)\sqrt{2}\approx1.06$, which is within 10 percent of the numerically determined value.} %\MM{well, the absolute energy eigenvalue is probably not so relevant. As we are interested in the spacing between the levels. The latter seems to have an error of 10 percent. Better comment about this, too.}}

\subsubsection{{Center of the scar spectrum}}
{We can also estimate the energy in the middle of the spectrum in the large $N_b$ limit. As an example, we estimate $E_1$. From Eq.~\eqref{c2_1}, $|c_{\pm2}|^2$ is expressed as}
\begin{equation}
\label{c2s}
\begin{split}
    {|c_2|^2}&{=\prod_{M=0}^{N_b-2}{\left((N_b-2)(N_b-1)-M(M-1)\right),\,|c_{-2}|^2=\prod_{M=0}^3(N_b-1-M)^2\prod_{M=4}^{N_b-2}\left((N_b-2)(N_b-1)-M(M-1)\right)}}.
    \end{split}
\end{equation}
{From this  one easily finds {$(|c_2|^2-|c_{-2}|^2)/|c_2|^2= 8/N_b+O(1/N_b^2)$} in the large $N_b$ limit. Using Eqs.~(\ref{norm}) and (\ref{c2s}), taking a logarithm and approximating the summation by an integral, one obtains $|c_2|^2/\mc{N}_1 = 1/16 +O(1/N_b)$.} Substituting these values into Eq.~\eqref{eq:energy correction formula}, the energy correction is estimated in the large $N_b$ limit as
\begin{equation}
    {\Delta E_1\approx-\frac{\sqrt{2}}{8}N_b\frac{8}{N_b}\times\frac{1}{16}=-\frac{\sqrt{2}}{16}.}
\end{equation}
Recalling that $E_0=0$, This yields an estimate of the level spacing in the centrum of the scar spectrum as $\Delta E_{\rm center}= E_1 \approx \sqrt{2}+ \Delta E_1= 15\sqrt{2}/16$.

\subsection{The middle of the spectrum using $\ket*{\mr{MPS}_n}$}\label{app:MPS ansatz}
To estimate the energy of $\ket*{\mc{S}_1^{\mr{PXP}}}$, we use the alternative ansatz $\ket*{\mr{MPS}_1}$ in Eq.~\eqref{eq:|MPS>}. Using the MPS representation, $\ket*{\mr{MPS}_1}$ can be written as
\begin{equation}
\label{MPS}
    \ket*{\mr{MPS}_1}=\sum_{b\in\Lambda_{\mr{B}}}\sum_{\{\sigma_i\}_{i=1}^N\in\{\pm,0\}^{\otimes N}}P_{\mr{Ryd}}\left(\msf{v}_\rightarrow^{\sigma_b}\right)^{\mr{T}}\msf{A}^{\sigma_{[b+1]}}\cdots\msf{A}^{\sigma_{[b+N-2]}}\msf{w}_\rightarrow^{\sigma_{[b+N-1]}}\ket*{\sigma_1\cdots\sigma_N},
\end{equation}
where $[b]$ satisfies $b\equiv[b] (\mr{mod}\,\,N)$ and $1\leq [b]<N$. This is conveniently rewritten by defining the wavefunction  $\ket*{M^{\rightarrow\rightarrow}_{b,b+1}}$  as
\begin{equation}\begin{split}
    %\ket*{\wtil{\mr{MPS}}_1}&\coloneqq\sum_{b\in\Lambda_{\mr{B}}}\sum_{\{\sigma_i\}_{i=1}^N\in\{\pm,0\}^{\otimes N}}\left(\msf{v}_\rightarrow^{\sigma_b}\right)^{\mr{T}}\msf{A}^{\sigma_{[b+1]}}\cdots\msf{A}^{\sigma_{[b+N-2]}}\msf{w}_\rightarrow^{\sigma_{[b+N-1]}}\ket*{\sigma_1\cdots\sigma_N}\\
    \ket*{M^{\rightarrow\rightarrow}_{b,b+1}}&\coloneqq\sum_{\{\sigma_i\}_{i=1}^N\in\{\pm,0\}^{\otimes N}}\left(\msf{v}_\rightarrow^{\sigma_b}\right)^{\mr{T}}\msf{A}^{\sigma_{[b+1]}}\cdots\msf{A}^{\sigma_{[b+N-2]}}\msf{w}_\rightarrow^{\sigma_{[b+N-1]}}\ket*{\sigma_1\cdots\sigma_N}\\
    &=\msf{A}\ket*{\rightarrow\rightarrow}_{(b,\mr{R}),(b+1,\mr{L})}\bigotimes_{b'\in\Lambda_{\mr{B}}\setminus\{b\}}\frac{1}{\sqrt{2}}\left(\ket*{\uparrow\uparrow}-\ket*{\downarrow\downarrow}\right)_{(b',\mr{R}),(b'+1,\mr{L})},
    \end{split}
\end{equation}
so that the unprojected MPS parent state is $\ket*{\wtil{\mr{MPS}}_1}=\sum_{b\in\Lambda_{\mr{B}}}\ket*{M^{\rightarrow\rightarrow}_{b,b+1}}$, and one has  $\ket*{\mr{MPS}_1}=P_{\mr{Ryd}}\ket*{\wtil{\mr{MPS}}_1}$ and .
With this we find
\begin{equation}\label{eq:H|S'1>}\begin{split}
    H\ket*{\mr{MPS}_1}&=\sqrt{2}\ket*{\mr{MPS}_1}-\sum_{b\in\Lambda_{\mr{B}}}P_{\mr{Ryd}}\left(\ket*{+,0}+\ket*{0,-}\right)\bra*{+,-}_{b,b+1}\ket*{M^{\rightarrow\rightarrow}_{b,b+1}}\\
    &=\sqrt{2}\ket*{\mr{MPS}_1}+\frac{1}{4}\sum_{b\in\Lambda_{\mr{B}}}\left(\ket*{+,0}+\ket*{0,-}\right)_{b,b+1}\otimes\ket*{M^{\uparrow\downarrow}_{b-1,b+2}},
    \end{split}
\end{equation}
where
\begin{equation}
    \begin{split}
        \ket*{M_{b-1,b+2}^{\uparrow\downarrow}}\coloneqq\left(\bigotimes_{b'\in\Lambda_{\mr{B}}\setminus\{b,b+1\}}A_{b'}\right)\ket*{\uparrow\downarrow}_{(b-1,\mr{R}),(b+2,\mr{L})}\bigotimes_{b''\in\Lambda_{\mr{B}}\setminus\{b-1,b,b+1\}}\frac{1}{\sqrt{2}}\left(\ket*{\uparrow\uparrow}-\ket*{\downarrow\downarrow}\right)_{(b'',\mr{R}),(b''+1,\mr{L})}.
    \end{split}
\end{equation}
The MPS representation of $\ket*{M^{\uparrow\downarrow}_{b-1,b+2}}$ is as follows:
\begin{equation}
    \ket*{M_{b-1,b+2}^{\uparrow\downarrow}}=\sum_{\{\sigma_i\}_{i\in\Lambda_{B}\setminus\{b,b+1\}}\in\{\pm,0\}^{\otimes N-2}}\left(\msf{v}^{\sigma_{[b+2]}}_\downarrow\right)^{\mr{T}}\msf{A}^{\sigma_{[b+3]}}\cdots\msf{A}^{\sigma_{[b-2]}}\msf{w}_\uparrow^{\sigma_{[b-1]}}\ket*{\sigma_1\cdots\sigma_{N}},
\end{equation}
where $\sigma_b$ and $\sigma_{b+1}$ are excluded from the summation. We have defined the boundary vectors as $\msf{v}_\downarrow^\sigma\coloneqq(\msf{v}^\sigma_\rightarrow-\msf{v}^\sigma_\leftarrow)/\sqrt{2}$ and $\msf{w}^\sigma_\uparrow\coloneqq(\msf{w}^\sigma_\rightarrow+\msf{w}^\sigma_\leftarrow)/\sqrt{2}$. We denote the second term in the second line in Eq.~\eqref{eq:H|S'1>} as $\ket*{\delta\mr{MPS}_1}$, i.e., $H\ket*{\mr{MPS}_1}=\sqrt{2}\ket*{\mr{MPS}_1}+\frac{1}{4}\ket*{\delta\mr{MPS}_1}$. Thus, the energy expectation value of $\ket*{\mr{MPS}_1}$ can be evaluated from 
\begin{equation}\label{eq:renormalized H|S'1>}
    H\ket*{\mr{MPS}_1}=\left(\sqrt{2}+\frac{1}{4}\frac{\innerproduct*{\mr{MPS}_1}{\delta\mr{MPS}_1}}{\innerproduct*{\mr{MPS}_1}{\mr{MPS}_1}}\right)\ket*{\mr{MPS}_1}+\ket*{\mr{MPS}_\perp},
\end{equation}
where $\ket*{\mr{MPS}_\perp}$ satisfies $\innerproduct*{\mr{MPS}_1}{\mr{MPS}_\perp}=0$. Since both $\ket*{\mr{MPS}_1}$ and $\ket*{\delta\mr{MPS}_1}$ can be expressed as MPS, one can calculate their norm and inner product by standard techniques for MPS states. %We omit a detailed derivation here, 
For large $N$ one finds,
\begin{equation}
    \innerproduct*{\mr{MPS}_1}\cong\frac{14N}{9}\left(\frac{3}{4}\right)^N,\,\,\innerproduct*{\mr{MPS}_1}{\delta\mr{MPS}_1}\cong-\frac{4\sqrt{2}N}{9}\left(\frac{3}{4}\right)^N.
\end{equation}
Thus, for large $N$, we obtain $\sqrt{2}+\frac{1}{4}\frac{\innerproduct*{\mr{MPS}_1}{\delta\mr{MPS}_1}}{\innerproduct*{\mr{MPS}_1}}\cong\frac{13}{14}\sqrt{2}\cong1.3132$, which is indeed very close to the empirical level spacing ($\Omega_{\rm PXP}\cong1.33$) between scar states close to the center of the spectrum.

To quantify the quality of the approximation of the trial scar state, one can estimate $\norm*{\ket*{\mr{MPS}_\perp}}$ and obtains $\norm*{\ket*{\mr{MPS}_\perp}}/\norm*{\ket*{\mr{MPS}_1}}=\sqrt{151/(3\cdot14^3)}\cong0.1354$ in the thermodynamic limit.  

\section{Estimate of optimal  scar-enhancement}
In the main text we have quoted the optimal coefficient for the perturbation $\delta H(\lambda)$ (Eq.~\eqref{eq:dH2new(lambda)}). Here we provide a detailed derivation.
The actual goal is to minimize $\sum_n\norm*{P_{\mr{Ryd}}(H_1+\delta H(\lambda))\ket*{S_n}}^2$ with respect to $\lambda$, which we carried out numerically for $N=10$ blocks. Here, we instead want to gain more analytical understanding. 
To keep the task tractable we drop the projection on the Rydberg subspace and restrict ourselves to  minimizing $\sum_n\norm*{(H_1+\delta H(\lambda))\ket*{\wtil{S}_n}}^2$, under the assumption that the two optimization problems do not differ too much.

\subsection{The scar states}
The trial wave function $\ket{S_n}$ for the $n$'th scar state is as follows,
\begin{equation}\begin{split}
    \ket{S_n}&=P_{\mr{Ryd}}\ket*{\wtil{S}_n}=P_{\mr{Ryd}}\left(J^-\right)^{N-n}\bigotimes_{b\in\Lambda_{\mr{B}}}\ket*{\what{+}}_b
    \\
    J^\pm&=\sqrt{2}\sum_{b\in\Lambda_{\mr{B}}}\left(\dyad*{\what{\pm}}{\what{0}}+\dyad*{\what{0}}{\what{\mp}}\right)_b.
    \end{split}
\end{equation}
We split the collective spin-raising (lowering) operator as
\begin{equation}\begin{split}
    J^\pm&=J_{b,b+1}^\pm+J_{\Lambda_{\mr{B}}\setminus\{b,b+1\}}^\pm\\
    J_{b,b+1}^\pm&\coloneqq\sqrt{2}\left(\dyad*{\what{\pm}}{\what{0}}+\dyad*{\what{0}}{\what{\mp}}\right)_b+\sqrt{2}\left(\dyad*{\what{\mp}}{\what{0}}+\dyad*{\what{0}}{\what{\mp}}\right)_{b+1}\\
    J^\pm_{\Lambda_{\mr{B}}\setminus\{b,b+1\}}&\coloneqq\sqrt{2}\sum_{b'\in\Lambda_{\mr{B}}\setminus\{b,b+1\}}\left(\dyad*{\what{\pm}}{\what{0}}+\dyad*{\what{0}}{\what{\mp}}\right)_{b'}.
    \end{split}
\end{equation}
Using these operators, we can write $\ket*{\wtil{S}_{N-n}}$ with $n\geq3$ as
\begin{equation}\begin{split}
    \ket*{\wtil{S}_{N-n}}&=\sum_{k=0}^4\binom{n}{k}\left(J^-_{b,b+1}\right)^k\ket*{\what{T}_{2,2}}_{b,b+1}\otimes\left(J^-_{\Lambda_{\mr{B}}\setminus\{b,b+1\}}\right)^{n-k}\ket*{\what{T}_{N-2,N-2}}_{\Lambda_{\mr{B}}\setminus\{b,b+1\}}\\
    &=c\ket*{\what{T}_{2,2}}_{b,b+1}\otimes\ket*{\what{T}_{N-2,N-n-2}}_{\Lambda_{\mr{B}}\setminus\{b,b+1\}}+2c\sqrt{\frac{n}{-n+2N-3}}\ket*{\what{T}_{2,1}}_{b,b+1}\otimes\ket*{\what{T}_{N-2,N-n-1}}_{\Lambda_{\mr{B}}\setminus\{b,b+1\}}\\
    &+c\sqrt{\frac{3n!(-n+2N-4)!}{2(n-2)!(-n+2N-2)!}}\ket*{\what{T}_{2,0}}_{b,b+1}\otimes\ket*{\what{T}_{N-2,N-n}}_{\Lambda_{\mr{B}}\setminus\{b,b+1\}}\\
    &+c\sqrt{\frac{n!(-n+2N-4)!}{6(n-3)!(-n+2N-1)!}}\ket*{\what{T}_{2,-1}}_{b,b+1}\otimes\ket*{\what{T}_{N-2,N-n+1}}_{\Lambda_{\mr{B}}\setminus\{b,b+1\}}\\
    &+c\sqrt{\frac{n!(-n+2N-4)!}{(n-4)!(-n+2N)!}}\ket*{\what{T}_{2,-2}}_{b,b+1}\otimes\ket*{\what{T}_{N-2,N-n+2}}_{\Lambda_{\mr{B}}\setminus\{b,b+1\}},
    \end{split}
\end{equation}
where $c\coloneqq\prod_{M=N-n-1}^{N-2}\sqrt{(N-2)(N-1)-M(M-1)}$. Here, $\ket*{\what{T}_{S,M}}$ is a state with total spin $S$ and $S^x=M$. When $N$ is sufficiently large, one can approximate $\ket*{\wtil{S}_n}$ as
\begin{equation}\label{eq:|Sn> approximate}
    \begin{split}
        \frac{1}{c}\ket*{\wtil{S}_{N-n}}&\cong \ket*{\what{T}_{2,2}}_{b,b+1}\otimes\ket*{\what{T}_{N-2,N-n-2}}_{\Lambda_{\mr{B}}\setminus\{b,b+1\}}+2\sqrt{\frac{s}{2-s}}\ket*{\what{T}_{2,1}}_{b,b+1}\otimes\ket*{\what{T}_{N-2,N-n-1}}_{\Lambda_{\mr{B}}\setminus\{b,b+1\}}\\
        &+\sqrt{\frac{3}{2}}\frac{s}{2-s}\ket*{\what{T}_{2,0}}_{b,b+1}\otimes\ket*{\what{T}_{N-2,N-n}}_{\Lambda_{\mr{B}}\setminus\{b,b+1\}}+\sqrt{\frac{s^3}{6(2-s)^3}}\ket*{\what{T}_{2,-1}}_{b,b+1}\otimes\ket*{\what{T}_{N-2,N-n+1}}_{\Lambda_{\mr{B}}\setminus\{b,b+1\}}\\
        &+\frac{1}{12}\frac{s^2}{(2-s)^2}\ket*{\what{T}_{2,-2}}_{b,b+1}\otimes\ket*{\what{T}_{N-2,N-n+2}}_{\Lambda_{\mr{B}}\setminus\{b,b+1\}},
    \end{split}
\end{equation}
where $s\coloneqq n/N$. Each coefficient is plotted in Fig.~\ref{fig:coeffs}. When $n$ is small, the dominant contribution in $\ket*{\wtil{S}_{N-n}}$ is $\ket*{\what{T}_{2,2}}_{b,b+1}$, but as $n$ increases $\ket*{\what{T}_{2,1}}_{b,b+1}$ and $\ket*{\what{T}_{2,0}}_{b,b+1}$ become dominant. For later arguments, we define the reduced density matrix $\rho_S$ for the incoherent equal weight distribution over the states $\ket*{\wtil{S}_n}$ as 
\begin{equation}
    \rho_S\coloneqq\frac{1}{N}\sum_{n=1}^N\mr{Tr}_{\Lambda_{\mr{B}}\setminus\{b,b+1\}}\frac{1}{\norm*{\ket*{\wtil{S}_n}}^2}\dyad*{\wtil{S}_n},
\end{equation}
where $\mr{Tr}_{\Lambda_{\mr{B}}\setminus\{b,b+1\}}$ is a partial trace on $\Lambda_{\mr{B}}\setminus\{b,b+1\}$. We can approximately obtain $\rho_S$ using Eq.~\eqref{eq:|Sn> approximate} as
\begin{equation}
    \begin{split}
        \rho_S&\cong\frac{1}{N}\sum_{s=1/N}^{1}\frac{1}{Z(s)}\left(P^{(2,2)}_{b,b+1}+\frac{4s}{2-s}P^{(2,1)}_{b,b+1}+\frac{3s^2}{2(2-s)^2}P^{(2,0)}_{b,b+1}+\frac{s^3}{6(2-s)^3}P^{(2,-1)}_{b,b+1}+\frac{s^4}{144(2-s)^4}P^{(2,-2)}_{b,b+1}\right)\\
        Z(s)&\coloneqq1+\frac{4s}{2-s}+\frac{3s^2}{2(2-s)^2}+\frac{s^3}{6(2-s)^3}+\frac{s^4}{144(2-s)^4},
    \end{split}
\end{equation}
where $P_{b,b+1}^{(S,M)}\coloneqq\dyad*{\what{T}_{S,M}}_{b,b+1}$. We can approximate $\rho_S$ further by replacing $N^{-1}\sum_{s=1/N}^1\rightarrow\int_0^1ds$.
\begin{figure}
    \centering
    \includegraphics[width=.5\textwidth]{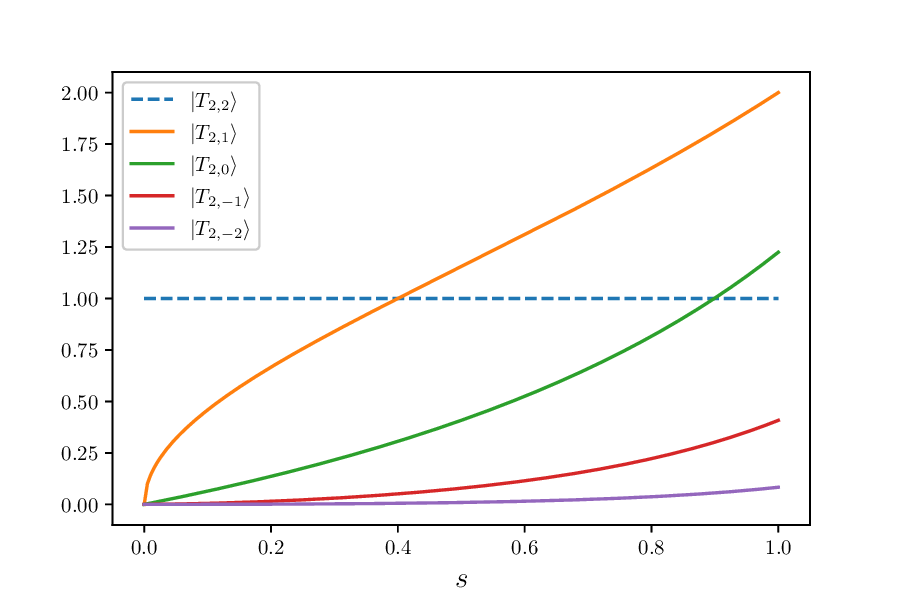}
    \caption{Coefficients of $\ket*{\what{T}_{2,M}} (-2\leq M\leq 2)$ in Eq.~\eqref{eq:|Sn> approximate} as functions of $s$.}
    \label{fig:coeffs}
\end{figure}
%\subsection{it Another trial wave functions}

\subsection{Estimate of the optimal perturbation strength $\lambda$}
As stated in the main text, we have 
\begin{equation}
    \begin{split}
        (H+\delta H(\lambda))\ket*{S_n}&=P_{\mr{Ryd}}\left(H_{\mr{Z}}+H_{\mr{rem}}(\lambda)\right)\ket*{\wtil{S}_n},\\
        H_{\mr{rem}}(\lambda)&=\sum_{b\in\Lambda_{\mr{B}}}h_{b,b+1}(\lambda),\\
        h_{b,b+1}(\lambda)&=\frac{-1+2\lambda}{\sqrt{6}}\left(\ket*{+,0}+\ket*{0,-}\right)\bra*{T_{2,0}}_{b,b+1}+\frac{\lambda}{\sqrt{2}}\ket*{0,0}\left(\bra*{T_{2,1}}+\bra*{T_{2,-1}}\right)_{b,b+1}.
    \end{split}
\end{equation}
Thus, we find
\begin{equation}
    h_{b,b+1}^\dag(\lambda)h_{b,b+1}(\lambda)=\frac{(-1+2\lambda)^2}{3}\dyad*{T_{2,0}}_{b,b+1}+\frac{\lambda^2}{2}\left(\ket*{T_{2,1}}+\ket*{T_{2,-1}}\right)\left(\bra*{T_{2,1}}+\bra*{T_{2,-1}}\right)_{b,b+1}.
\end{equation}
As $\ket*{T_{2,0}}=\sqrt{3/8}\ket*{\what{T}_{2,2}}-1/2\ket*{\what{T}_{2,0}}+\sqrt{3/8}\ket*{\what{T}_{2,-2}}$ and $\ket*{T_{2,1}}+\ket*{T_{2,-1}}=\ket*{\what{T}_{2,2}}-\ket*{\what{T}_{2,-2}}$, we find
\begin{equation}
    \begin{split}
        \mr{Tr}_{\{b,b+1\}}\rho_Sh^\dag_{b,b+1}(\lambda)h_{b,b+1}(\lambda)&=\frac{(-1+2\lambda)^2}{3}\left(\frac{3}{8}\expval*{\rho_S}{\what{T}_{2,2}}+\frac{1}{4}\expval*{\rho_S}{\what{T}_{2,0}}+\frac{3}{8}\expval*{\rho_S}{\what{T}_{2,-2}}\right)\\
        &+\frac{\lambda^2}{2}\left(\expval*{\rho_S}{\what{T}_{2,2}}+\expval*{\rho_S}{\what{T}_{2,-2}}\right)\\
        &\cong\frac{1}{N}\sum_{s=1/N}^1\left[\frac{(-1+2\lambda)^2}{8Z(s)}\left(1+\frac{s^2}{(2-s)^2}+\frac{s^4}{144(2-s)^4}\right)+\frac{\lambda^2}{2Z(s)}\left(1+\frac{s^4}{144(2-s)^4}\right)\right]\\
        &\cong\int_0^1ds\left[\frac{(-1+2\lambda)^2}{8Z(s)}\left(1+\frac{s^2}{(2-s)^2}+\frac{s^4}{144(2-s)^4}\right)+\frac{\lambda^2}{2Z(s)}\left(1+\frac{s^4}{144(2-s)^4}\right)\right],
    \end{split}
\end{equation}
where $\mr{Tr}_{\{b,b+1\}}$ is the partial trace over the degrees of freedom on $\{b,b+1\}$. This function becomes smallest at $\lambda=\alpha/(2(\alpha+\beta))$, where
\begin{equation}\label{eq:alpha, beta}
    \begin{split}
        \alpha&\coloneqq\int_0^1ds\frac{1}{Z(s)}\left(1+\frac{s^2}{(2-s)^2}+\frac{s^4}{144(2-s)^4}\right)\cong0.5350,\\
        \beta&\coloneqq\int_0^1ds\frac{1}{Z(s)}\left(1+\frac{s^4}{144(2-s)^4}\right)\cong0.4739.
    \end{split}
\end{equation}
Thus, we find the optimal coefficient $\lambda\cong0.2651$. We define integrands in Eq.~\eqref{eq:alpha, beta} as $\alpha(s)$ and $\beta(s)$, i.e., $\alpha=\int_0^1ds\alpha(s), \beta=\int_0^1ds\beta(s)$.% \MM{I would not show this plot. What does it reveal?} and plot them in Fig.~\ref{fig:integrand}.
